# Supplementary material for: Anomalous contribution to the nematic electronic states from the structural transition in FeSe revealed by time- and angle-resolved photoemission spectroscopy
Source: arXiv:2206.06781 source file (2022-06-14)
Supplement: Supplementary file 1 [file FeSe-trARPES-SM.pdf]

# Anomalous contribution to the nematic electronic states from the structural transition in FeSe revealed by time- and angle-resolved photoemission spectroscopy: supplemental material

Yuanyuan Yang,[1] Qisi Wang,[2] Shaofeng Duan,[1] Hongliang Wo,[2] Chaozhi Huang,[1] Shichong Wang,[1] Lingxiao Gu,[1] Dao Xiang,[3,4] Dong Qian,[1,4,5] Jun Zhao,[2,6] and Wentao Zhang[1,4,5,*]

[1]*Key Laboratory of Artificial Structures and Quantum Control (Ministry of Education), Shenyang National Laboratory for Materials Science, School of Physics and Astronomy, Shanghai Jiao Tong University, Shanghai 200240, China*
[2]*State Key Laboratory of Surface Physics and Department of Physics, Fudan University, Shanghai 200433, China*
[3]*Key Laboratory for Laser Plasmas (Ministry of Education), School of Physics and Astronomy, Shanghai Jiao Tong University, Shanghai 200240, China*
[4]*Tsung-Dao Lee Institute, Shanghai Jiao Tong University, Shanghai 200240, China*
[5]*Collaborative Innovation Centreof Advanced Microstructures, Nanjing University, Nanjing 210093, China*
[6]*Institute of Nanoelectronics and Quantum Computing, Fudan University, Shanghai 200433, China*

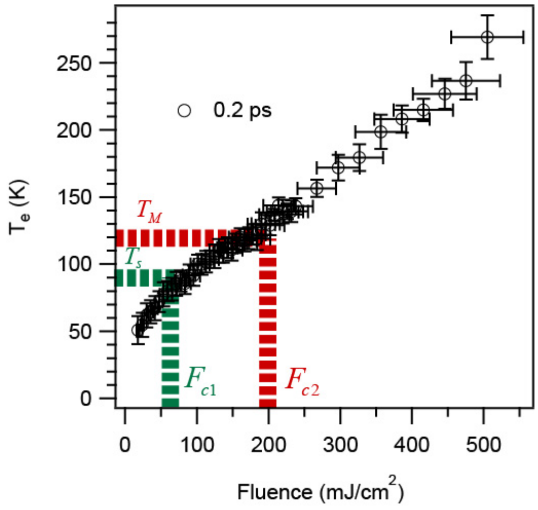


Supplemental FIG. 1. Electronic temperature, obtained by fitting the momentum-integrated spectra to an energy resolution convolved Fermi distribution function, as a function of pump fluence for the delay time at 0.2 ps.

*wentaozhang@sjtu.edu.cn

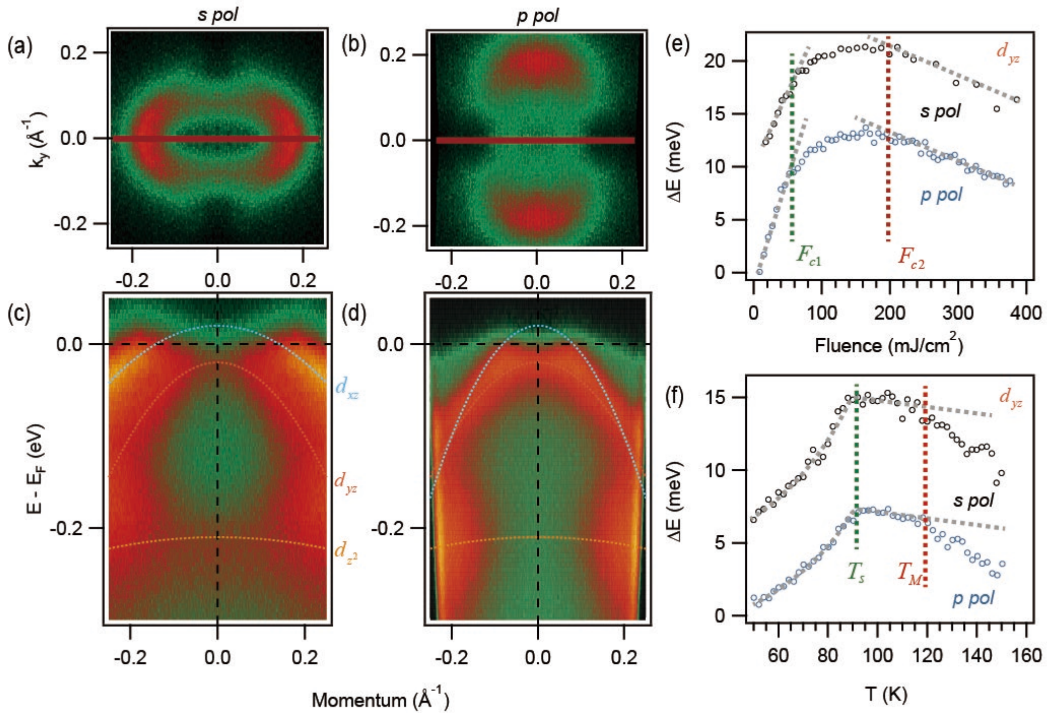


Supplemental FIG. 2. Fluence- and temperature-dependent measurements on two different spots. (a) and (b), photoemission mapping at the Fermi energy for s- and p-polarized probe (two different spots), respectively. (c) and (d), the photoemission spectra from the cuts shown in (a) and (b), respectively. (e) and (f), Pump fluence and temperature dependent energy shift of the $d_{yz}$ bands for the two cuts in (a) and (b), respectively.

**Supplemental Discussion #1**

To elaborate the $F_{c1}$ and $F_{c2}$ appearing in the ultrafast measurement more clearly, we estimated the transient electronic temperature ($T_e$) by fitting the momentum-integrated EDCs to Fermi-Dirac functions convoluted by the instrumental resolution (Supplemental FIG. 1). After the photoexcitation ~ 0.2 ps, $T_e$ increases as enhancing the optical excitation fluence, and it shows that $T_e$ at $F_{c1}$ and $F_{c2}$ are consistent with the $T_s$ (~90 K) and $T_M$ (~120 K), respectively, within error bars. Since the nematic phase and orbital order are purely electronic origin, there should be transitions with enhancing the electronic temperature with ultrafast photoexcitation. The quantitatively consistence between the transient electronic temperatures at the $F_{c1}$ and $F_{c2}$ and the equilibrium transition temperatures $T_s$ and $T_M$ strongly suggests that the $F_{c1}$ and $F_{c2}$ are the two critical pump fluences driving the two electronic phase transitions.

**Supplemental Discussion #2**

It is generally believed that in FeSe there is an orbital order, which corresponds to the degeneracy of $d_{xz}$ and $d_{yz}$ orbits (50~60 meV) at a specific temperature, and the orbital order is the driven force of the nematic phase transition at $T_s$. Such a degeneracy of $d_{xz}$ and $d_{yz}$ orbits has been widely confirmed at M point from equilibrium ARPES experiments ([S1]–[S4]). However, some results suggest that the temperature of the degeneracy and the nematic phase transition are at a similar temperature ([S1], [S2]), while some publications suggest a higher temperature for the degeneracy than the $T_s$ ([S3], [S4]). Such a degeneracy at $T_M$ is also evidenced in the few-layer FeSe sample ([S5], [S6]). The temperature scale associated with the degeneracy of $d_{xz}$ and $d_{yz}$ bands is also evidenced near the Gamma point ([S5]).

From previous studies, the $T_M$ is the critical temperature of the formation of the orbital order, and the order parameter associated in the transition can be the band gap between the $d_{xz}$ and $d_{yz}$ bands ([S7],[S8]).

In the modified Fig. 4(a), the kink feature at $T_M$ is robust in different samples, different momentum cut directions, and different probe photon energies. To our knowledge, it is the first time to identify both the $T_M$ and $T_s$ in a single temperature dependent band evolution (Figure 4), strongly suggesting that there is another temperature scale above the nematic transition temperature $T_s$. Importantly, the value of the $T_M$ from the measurement near the Gamma point here is consistent with that the recent studies at the M point.

However, the $T_M$ has not ever been evidenced in the transport measurements. It is possibly due to the fact that the band gap is tens of meV below the Fermi energy and it has less contribution to the conduct carriers, making it is hard to resolve the $T_M$ experimentally in transport measurement. In a recent study, $T_M$ was signatured as a peak in the $d\rho/dT$ curve but not discussed ([S9]).

**Supplemental Discussion #3**

In Supplemental FIG. 2, we show the measurements on two different spots, and we also used s- and p-polarized incident light to minimize the possible intensity contribution from the other domains, which are twofold symmetric and elliptical, rotated to each other by 90° and elongated along the X and Y directions, respectively. The corresponding band structures along the high-symmetry degree, labelled by dark red cuts in panels (a) and (b), are displayed in panels (c) and (d). We can see that in the *p-pol* measurements, only information of $d_{yz}$-orbit characterized band could be extracted due to the weak spectral weight contribution for the $d_{xz}$ - and $d_{z2}$ - orbit bands. We took additional fluence- and temperature-dependent measurements on the two domains in panels (e) and (f), in which the results show good consistence between the two cuts for both of the fluence and temperature dependent measurements.


[S1] M. D. Watson, T. K. Kim, A. A. Haghighirad, N. R. Davies, A. McCollam, A. Narayanan, S. F. Blake, Y. L. Chen, S. Ghannadzadeh, A. J. Schofield, M. Hoesch, C. Meingast, T. Wolf, and A. I. Coldea, Phys. Rev. B 91, 155106 (2015).

[S2] M. Yi, H. Pfau, Y. Zhang, Y. He, H. Wu, T. Chen, Z. R. Ye, M. Hashimoto, R. Yu, Q. Si, D.-H. Lee, P. Dai, Z.-X. Shen, D. H. Lu, and R. J. Birgeneau, Phys. Rev. X 9, 041049 (2019).

[S3] K. Nakayama, Y. Miyata, G. N. Phan, T. Sato, Y. Tanabe, T. Urata, K. Tanigaki, and T. Takahashi, Phys. Rev. Lett. 113, 237001 (2014).

[S4] P. Zhang, T. Qian, P. Richard, X. P. Wang, H. Miao, B. Q. Lv, B. B. Fu, T. Wolf, C. Meingast, X. X. Wu, Z. Q. Wang, J. P. Hu, and H. Ding, Phys. Rev. B 91, 214503 (2015).

[S5] Y. Zhang, M. Yi, Z.-K. Liu, W. Li, J. J. Lee, R. G. Moore, M. Hashimoto, M. Nakajima, H. Eisaki, S.-K. Mo, Z. Hussain, T. P. Devereaux, Z.-X. Shen, and D. H. Lu, Phys. Rev. B 94, 115153 (2016).

[S6] S. Tan, Y. Zhang, M. Xia, Z. Ye, F. Chen, X. Xie, R. Peng, D. Xu, Q. Fan, H. Xu, J. Jiang, T. Zhang, X. Lai, T. Xiang, J. Hu, B. Xie, and D. Feng, Nat. Mater. 12, 634–640 (2013).

[S7] A. I. Coldea and M. D. Watson, Annu. Rev. Condens. Matter Phys. 9, 125–146 (2018).

[S8] R. Q. Xing, L. Classen, and A. V. Chubukov, Phys. Rev. B 98, 41108 (2018).

[S9] Q. Ma, F. Lan, X. Li, Z. Du, H. Li, and Z. Ma, Scr. Mater. 176, 88–93 (2020).
